# Supplementary material for: Graph-CoVis: GNN-based Multi-view Panorama Global Pose Estimation
Source: arXiv:2304.13201 source file (2023-04-26)
Supplement: Supplementary file 1 [file additional_ATE_plots.tex]

For the three-view setting, we study the error as a function of distance, rotation, and co-visibility of the panoramas with respect to the origin panorama.
Figure \ref{fig:ate_vs_mean_dist} shows the translation error (ATE) as a function of mean distance of the panoramas from the origin panorama. For easier comparison, the first and second order polynomial fits to the points in the three plots are shown in Figure~\ref{fig:ate_vs_mean_dist_curves}. Graph-Covis consistently out-performs CoVisPose+Greedy and CoVisPose+PGO baselines for all distances from the origin panorama.

\begin{figure*}[t]
  \centering
  % \fbox{\rule{0pt}{2in} \rule{0.9\linewidth}{0pt}}
    \includegraphics[width=.75\linewidth]{images/ATE_vs_X_plots/1_mean_origin_distance_error.png}
    \caption{Mean distance of panoramas to origin (x axis, meters) v/s ATE (y axis, meters) for CovisPose+Greedy, CovisPose+PGO, and Graph-Covis. The yellow and red curves are first and second order polynomial fits to the data points.} 
    \label{fig:ate_vs_mean_dist}
\end{figure*}

\begin{figure*}[t]
  \centering
  % \fbox{\rule{0pt}{2in} \rule{0.9\linewidth}{0pt}}
    \includegraphics[width=.8\linewidth]{images/ATE_vs_X_plots/1b_mean_origin_distance_interp_curves.png}
    \caption{First (left) and second (right) order polynomial fits to ATE values in Figure \ref{fig:ate_vs_mean_dist} show that Graph-Covis (green solid) consistently outperforms other baselines (dashed).}
    \label{fig:ate_vs_mean_dist_curves}
\end{figure*}

Figure~\ref{fig:ate_vs_mean_rot} shows the translation error (ATE) as a function of mean rotation of the panoramas compared to the origin panorama. Direct comparison of the curves in Figure~\ref{fig:ate_vs_mean_rot_curves} shows Graph-Covis consistently out-performs baselines for all rotation values. %from origin.

\begin{figure*}[t]
  \centering
  % \fbox{\rule{0pt}{2in} \rule{0.9\linewidth}{0pt}}
    \includegraphics[width=.75\linewidth]{images/ATE_vs_X_plots/4_mean_origin_rotation_error.png}
    \caption{Mean absolute rotation of panoramas to origin (x axis, degrees) v/s ATE (y axis, meters) for CovisPose+Greedy, CovisPose+PGO, and Graph-Covis. The yellow and red curves are first and second order polynomial fits to the data points.} 
    \label{fig:ate_vs_mean_rot}
\end{figure*}

\begin{figure*}[t]
  \centering
  % \fbox{\rule{0pt}{2in} \rule{0.9\linewidth}{0pt}}
    \includegraphics[width=.8\linewidth]{images/ATE_vs_X_plots/4b_mean_origin_rotation_interp_curves.png}
    \caption{First (left) and second (right) order polynomial fits to ATE values in Figure \ref{fig:ate_vs_mean_rot} show that Graph-Covis (green solid) consistently outperforms other baselines (dashed).}
    \label{fig:ate_vs_mean_rot_curves}
\end{figure*}

Finally, Figure~\ref{fig:ate_vs_mean_covis} shows the translation error (ATE) as a function of mean co-visibility of the panoramas compared to the origin panorama. Graph-Covis performs better than baselines for larger co-visibilities. Similar to Section~\ref{sec:generalize_graph_covis}, the distribution of training samples in Figure~\ref{fig:ate_covis_distribution} shows that there are very few training examples with low mean co-visibility. The performance of Graph-Covis may be improved in the lower co-visibility range by adding more training examples in this region.

\begin{figure*}[t]
  \centering
  % \fbox{\rule{0pt}{2in} \rule{0.9\linewidth}{0pt}}
    \includegraphics[width=.75\linewidth]{images/ATE_vs_X_plots/7_mean_origin_covis_error.png}
    \caption{Mean co-visibility of panoramas to origin (x axis, percentage) v/s ATE (y axis, meters) for CovisPose+Greedy, CovisPose+PGO, and Graph-Covis. The yellow and red curves are first and second order polynomial fits to the data points.} 
    \label{fig:ate_vs_mean_covis}
\end{figure*}

\begin{figure*}[t]
  \centering
  % \fbox{\rule{0pt}{2in} \rule{0.9\linewidth}{0pt}}
    \includegraphics[width=.8\linewidth]{images/ATE_vs_X_plots/7b_mean_origin_covis_interp_curves.png}
    \caption{First (left) and second (right) order polynomial fits to ATE values in Figure \ref{fig:ate_vs_mean_covis} show that Graph-Covis (green solid) outperforms other baselines (dashed) for higher values of co-visibility.}
    \label{fig:ate_vs_mean_covis_curves}
\end{figure*}

\begin{figure*}[t]
  \centering
  % \fbox{\rule{0pt}{2in} \rule{0.9\linewidth}{0pt}}
    \includegraphics[width=.5\linewidth]{images/ATE_vs_X_plots/7c_mean_origin_covis_density.png}
    \caption{Distribution of samples over different co-visibility values. The worse performance of Graph-CoVis for lower co-visibility examples in Figure \ref{fig:ate_vs_mean_covis_curves} is likely due to the low number of training examples in this region.}
    \label{fig:ate_covis_distribution}
\end{figure*}
